# Supplementary material for: A Private and Finite-Time Algorithm for Solving a Distributed System of Linear Equations
Source: arXiv:2004.04680 source file (2020-04-09)
Supplement: Supplementary file 1 [file appendix.tex]

\appendix
